# Supplementary material for: SPAM: Stateless Permutation of Application Memory
Source: arXiv:2007.13808 source file (2020-09-21)
Supplement: Supplementary file 1 [file security-appendix.tex]

\section{Additional Security}
\begin{patchcode}
\centering
\begin{minted}
  [
  linenos,
  fontsize=\scriptsize,
  mathescape,
  autogobble,
  stripall,
  breakbytokenanywhere=true,
  numbersep=3pt
  ]
  {diff}
diff --git a/nginx/src/http/ngx_http_parse.c
b/nginx/src/http/ngx_http_parse.c
--- a/nginx/src/http/ngx_http_parse.c
+++ b/nginx/src/http/ngx_http_parse.c
@@ -891,3 +891,3 @@ ngx_http_parse_header_line
  hash = ngx_hash(0, c);
- r->lowcase_header[0] = c;
+ r->p_lowcase_header->lowcase_header[0] = c;
  i = 1;
@@ -899,3 +899,3 @@ ngx_http_parse_header_line
  hash = ngx_hash(0, ch);
- r->lowcase_header[0] = ch;
+ r->p_lowcase_header->lowcase_header[0] = ch;
  i = 1;
@@ -926,3 +926,3 @@ ngx_http_parse_header_line
  hash = ngx_hash(hash, c);
- r->lowcase_header[i++] = c;
+ r->p_lowcase_header->lowcase_header[i++] = c;
  i &= (NGX_HTTP_LC_HEADER_LEN - 1);
@@ -934,3 +934,3 @@ ngx_http_parse_header_line
  hash = ngx_hash(hash, ch);
- r->lowcase_header[i++] = ch;
+ r->p_lowcase_header->lowcase_header[i++] = ch;
  i &= (NGX_HTTP_LC_HEADER_LEN - 1);
diff --git a/nginx/src/http/ngx_http_request.c
b/nginx/src/http/ngx_http_request.c
--- a/nginx/src/http/ngx_http_request.c
+++ b/nginx/src/http/ngx_http_request.c
@@ -927,2 +927,3 @@ ngx_http_process_request_line
  ngx_http_request_t  *r;
+ ngx_http_request_t_lowcase_header_t r_lowcase_header;
@@ -930,2 +931,3 @@ ngx_http_process_request_line
  r = c->data;
+ r->p_lowcase_header = &r_lowcase_header;
@@ -1196,2 +1198,3 @@ ngx_http_process_request_headers
  ngx_http_request_t         *r;
+ ngx_http_request_t_lowcase_header_t r_lowcase_header;
  ngx_http_core_srv_conf_t   *cscf;
@@ -1201,2 +1204,3 @@ ngx_http_process_request_headers
  r = c->data;
+ r->p_lowcase_header = &r_lowcase_header;
@@ -1311,3 +1315,3 @@ ngx_http_process_request_headers
  if (h->key.len == r->lowcase_index) {
-     ngx_memcpy(h->lowcase_key, r->lowcase_header, h->key.len);
+     ngx_memcpy(h->lowcase_key,
      r->p_lowcase_header->lowcase_header,
      h->key.len);
@@ -2187,2 +2191,3 @@ ngx_http_request_handler
  ngx_http_request_t  *r;
+ ngx_http_request_t_lowcase_header_t r_lowcase_header;
@@ -2190,2 +2195,3 @@ ngx_http_request_handler
  r = c->data;
+ r->p_lowcase_header = &r_lowcase_header;
@@ -2211,2 +2217,3 @@ ngx_http_run_posted_requests
  ngx_http_request_t         *r;
+ ngx_http_request_t_lowcase_header_t r_lowcase_header;
  ngx_http_posted_request_t  *pr;
@@ -2220,2 +2227,3 @@ ngx_http_run_posted_requests
  r = c->data;
+ r->p_lowcase_header = &r_lowcase_header;
  pr = r->main->posted_requests;
@@ -2268,2 +2276,3 @@ ngx_http_finalize_request
  ngx_http_request_t        *pr;
+ ngx_http_request_t_lowcase_header_t pr_lowcase_header;
  ngx_http_core_loc_conf_t  *clcf;
@@ -2351,2 +2360,3 @@ ngx_http_finalize_request
  pr = r->parent;
+ pr->p_lowcase_header = &pr_lowcase_header;
@@ -2456,2 +2466,3 @@ ngx_http_terminate_request
  ngx_http_request_t    *mr;
+ ngx_http_request_t_lowcase_header_t mr_lowcase_header;
  ngx_http_ephemeral_t  *e;
@@ -2459,2 +2470,3 @@ ngx_http_terminate_request
  mr = r->main;
+ mr->p_lowcase_header = &mr_lowcase_header;
@@ -3249,2 +3261,3 @@ ngx_http_lingering_close_handler
  ngx_http_request_t        *r;
+ ngx_http_request_t_lowcase_header_t r_lowcase_header;
  ngx_http_core_loc_conf_t  *clcf;
@@ -3254,2 +3267,3 @@ ngx_http_lingering_close_handler
  r = c->data;
+ r->p_lowcase_header = &r_lowcase_header;
@@ -3564,2 +3578,4 @@ ngx_http_log_error
  ngx_http_request_t  *r;
+ ngx_http_request_t_lowcase_header_t r_lowcase_header;
  ngx_http_log_ctx_t  *ctx;
@@ -3578,2 +3594,3 @@ ngx_http_log_error
  r = ctx->request;
+ r->p_lowcase_header = &r_lowcase_header;
diff --git a/nginx/src/http/ngx_http_request.h
b/nginx/src/http/ngx_http_request.h
--- a/nginx/src/http/ngx_http_request.h
+++ b/nginx/src/http/ngx_http_request.h
@@ -380,2 +380,6 @@ typedef void ... 
+ typedef struct {
+ u_char lowcase_header[32];
+ } ngx_http_request_t_lowcase_header_t;
+
 struct ngx_http_request_s {
@@ -566,3 +570,3 @@ struct ngx_http_request_s {
  ngx_uint_t lowcase_index;
- u_char     lowcase_header[NGX_HTTP_LC_HEADER_LEN];
+ ngx_http_request_t_lowcase_header_t *p_lowcase_header;
\end{minted}
\caption{\pname{} \b2p{} patch for Nginx to protect against pointer stretching
  attack as described in~\cite{Gil2018:Hole}.}
\label{lst:ngix-b2p-patch}
\end{patchcode}
